# Supplementary material for: Random survival forests with multivariate longitudinal endogenous covariates
Source: arXiv:2208.05801 source file (2023-02-09)
Supplement: Supplementary file 1 [file HAL_supp_v2.pdf]

# Supplementary material for Random survival forests with multivariate longitudinal endogenous covariates

Anthony Devaux[1], Catherine Helmer[1], Robin Genuer[1,2,*,†], and Cécile Proust-Lima[1,†]

[1]Univ. Bordeaux, INSERM, Bordeaux Population Health, UMR1219, Bordeaux, France

[2]INRIA Bordeaux Sud-Ouest, Talence, France

[*]Email: robin.genuer@u-bordeaux.fr

[†]These authors contributed equally to this work

January 2023

## 1 Simulations

### 1.1 Generating models

#### 1.1.1 Generation of the time-dependent markers

For all the scenarios, we generated repeated data for $m \in \{1, ..., M\}$ longitudinal markers using latent class linear mixed models ([1]) with $G = 4$ latent classes. The latent class-membership was first defined as a multinomial variable $c_{mi}$. Then, in each latent class $g$, the repeated measures at times $t_{ij}$ of marker $Y_{im}$ were generated according to the following model:

$$Y_{im}(t_{ij})|c_{mi} = g = \beta_{0gm} + \sum_{l=1}^{L-1} \beta_{lgm} * f_{ml}^{L}(t) + b_{i0m} + \sum_{l=1}^{L-1} b_{iml} * f_{ml}^{L}(t) + \epsilon_{ij}$$

The shape of the trajectory over time was defined according to a basis of natural cubic splines with $L$ knots $(f_{ml}^{L}(t))_{l=1,...,L-1}$. Depending on the marker and scenario, we chose among: (i) $L = 2$ resulting in a linear trajectory; (ii) $L = 3$ with one internal knot placed at $t = 5$; (iii) $L = 4$ with two internal knots placed at $t = 3$ and $t = 6$. The boundary knots were systematically placed

at $t = 0$ and $t = 10$. The basis of splines was associated with fixed effects $\beta_{lgm}$ to define the mean shape of the marker over time, and random effects $b_{im} = (b_{i0m}, b_{ilm})^\top \sim \mathcal{N}(0, D)$ to define individual departures from the class-specific mean trajectory. The measurement errors $\epsilon_{ij}$ were zero-mean independent Gaussian variables with variance $\sigma^2$.

Measurements times $t_{ij}$ were generated at baseline and were then randomly drawn around theoretical visits every year up to 10 years. Each year, a departure from the theoretical time was generated according an exponential distribution $\mathcal{E}(5)$.

#### 1.1.2 Generation of the time-to-event

We assumed a proportional hazard model for the time-to-event with instantaneous risk defined as:

$$\lambda_i(t) = \lambda_0(b, c, t) \exp(\mathcal{P}_i)$$

With $\lambda_0(b, c, t) = cb^c t^{c-1}$ the baseline hazard function from a Weibull distribution with parameters $b$ and $c$, and $\mathcal{P}_i$ the linear predictor. We fixed $b = 0.1$ and $c = 2$ for all scenarios.

### 1.2 Scenarios

A total of 4 scenarios were considered: 2 with $M = 2$ longitudinal predictors (called Small1, Small2) and 2 with $M = 20$ longitudinal predictors (called Large1, Large2). Details on the association between the predictors and event and associated parameters are given in table 1 for small scenarios and table 2 for large scenarios. An illustration of the longitudinal trajectories are given in figure 1 for the scenario with 2 predictors.

## 2 Applications

### 2.1 Individual prediction of dementia

Description and nature of the variables used in the application are detailed from Table 3 to Table 8. Several groups are also built using these variables (detailed in the same tables as indicated before).

Longitudinal trajectories are displayed in figure 2 for normalized clinical and neuropsychological predictors, in figure 3 for neuro-degenerative brain-MRI predictors and in figure 4 for normalized

vascular brain-MRI predictors.

Cumulative incidence functions of dementia and death are displayed in Figure 5 over the 20 years of follow-up.

To find the optimal $mtry$ value, we minimized the IBS criteria (see figure 6). We found that the lowest IBS value was for $mtry = 21$.

## References

[1] Proust-Lima, C., Séne, M., Taylor, J.M., Jacqmin-Gadda, H.: Joint latent class models for longitudinal and time-to-event data: A review. Statistical Methods in Medical Research **23**(1), 74–90 (2014). doi:10.1177/0962280212445839

# Figures

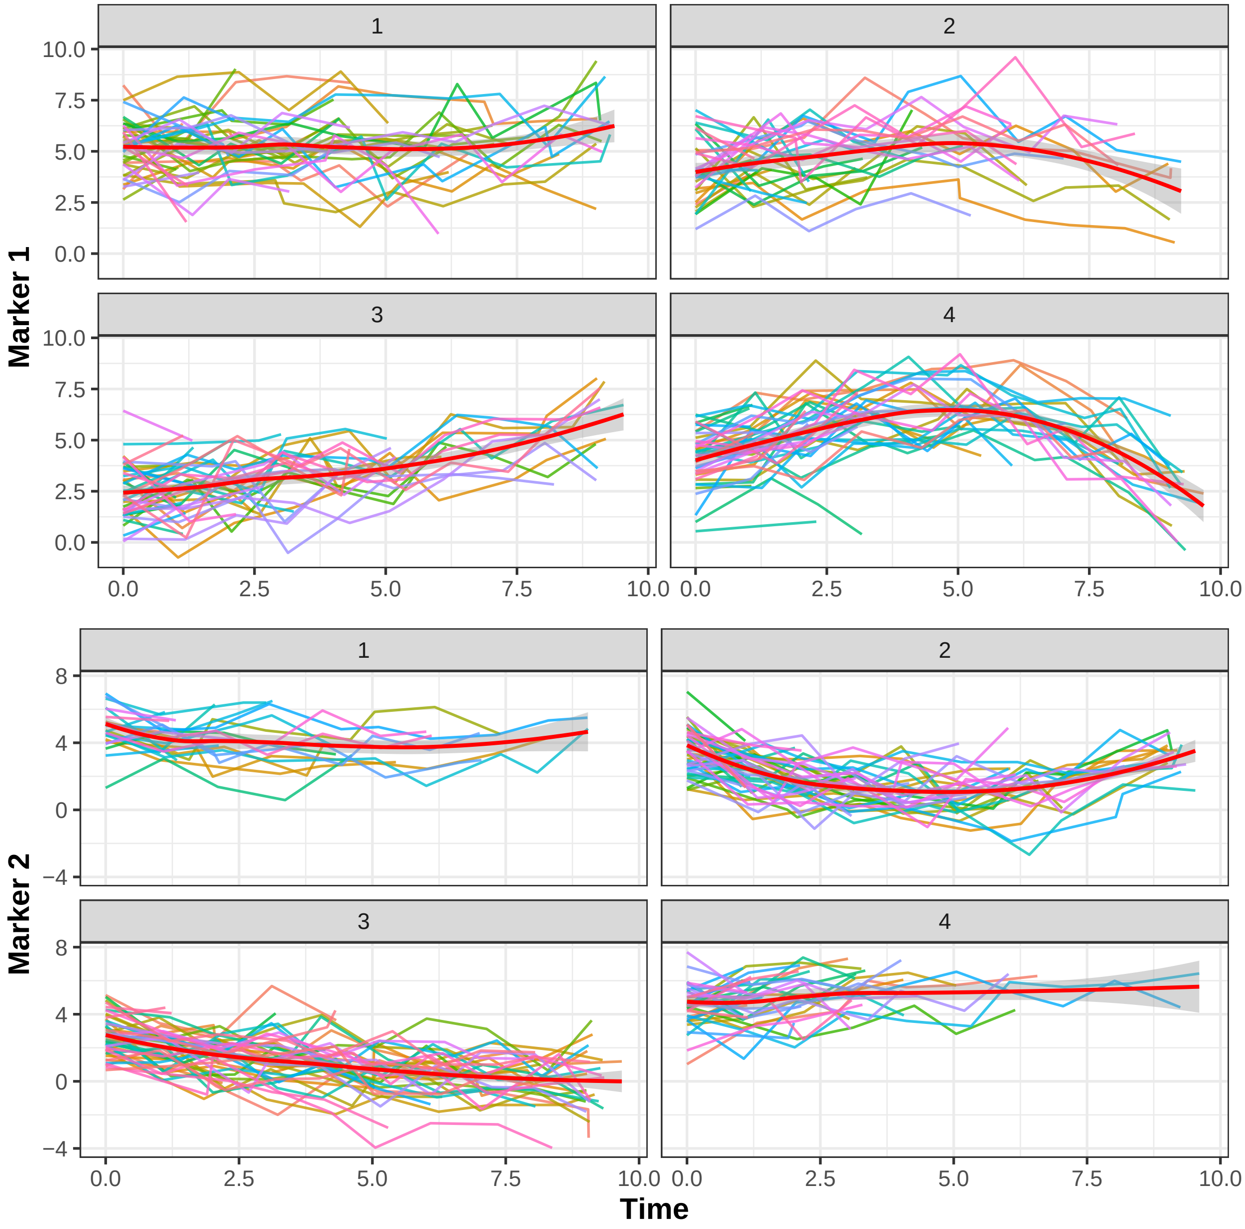


Figure 1: Illustration of 200 randomly selected individual trajectories chosen randomly for the two markers up to $t = 10$ in the first simulation study. Individual trajectories are displayed according to the four latent class specific to each marker. Bold red line indicates the mean trajectory given by smoothing method.

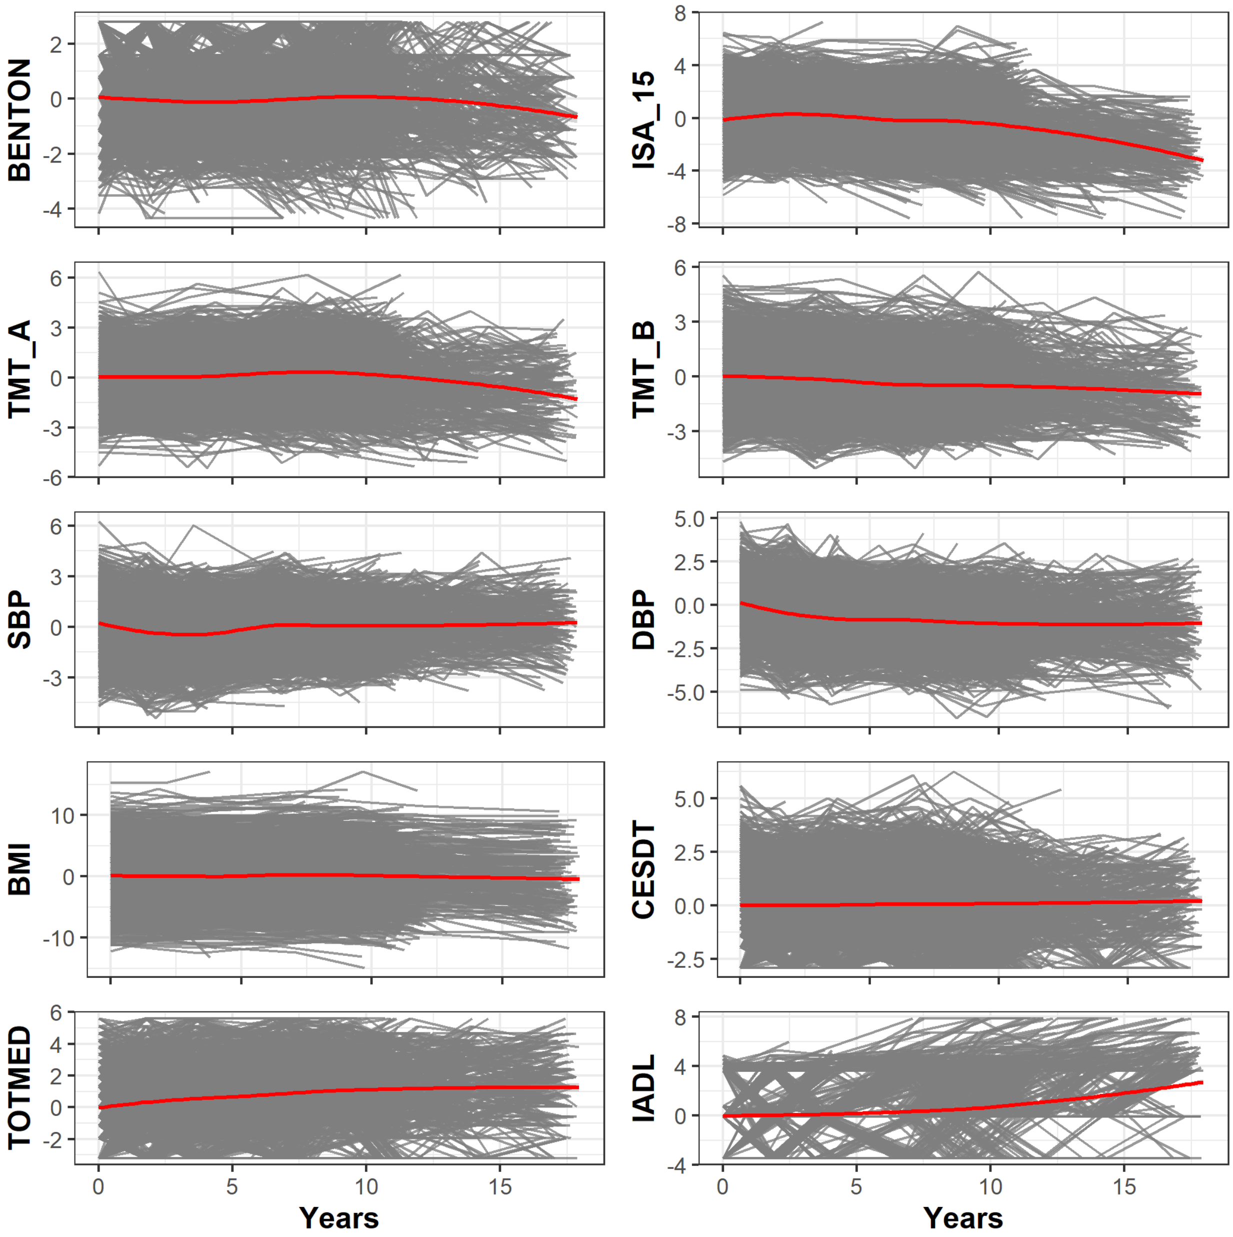


Figure 2: Individual trajectories from the normalized clinical and neuropsychological predictors in the 3C study. From left to right, we display the trajectories of Visual retention test of Benton, Isaac Set Test, Trail Making Test A, Trail Making Test B, Systolic Blood Pressure, Distolic Blood Pressure, Body-Mass Index, Depression symptoms, Number of drug consumed by day and Instrumental Activities of Daily Living.

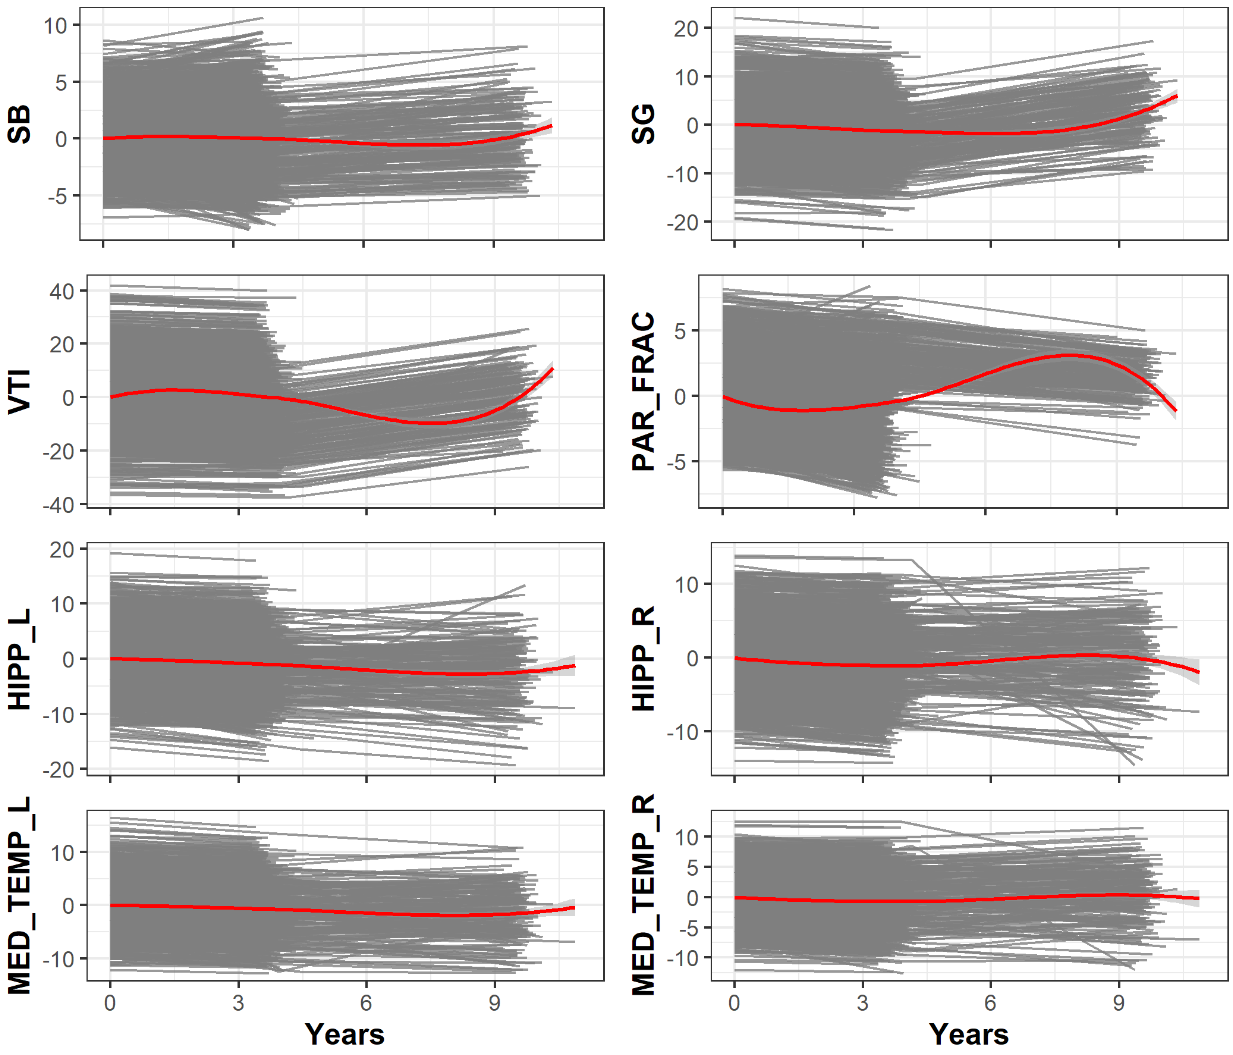


Figure 3: Individual trajectories from the normalized neuro-degenerative brain-MRI predictors in the 3C study. From left to right, we display the trajectories of white matter volume, grey matter volume, intracranial volume, parenchymal fraction, left hippocampal volume, right hippocampal volume, left mediotemporal lobe volume and right mediotemporal lobe volume.

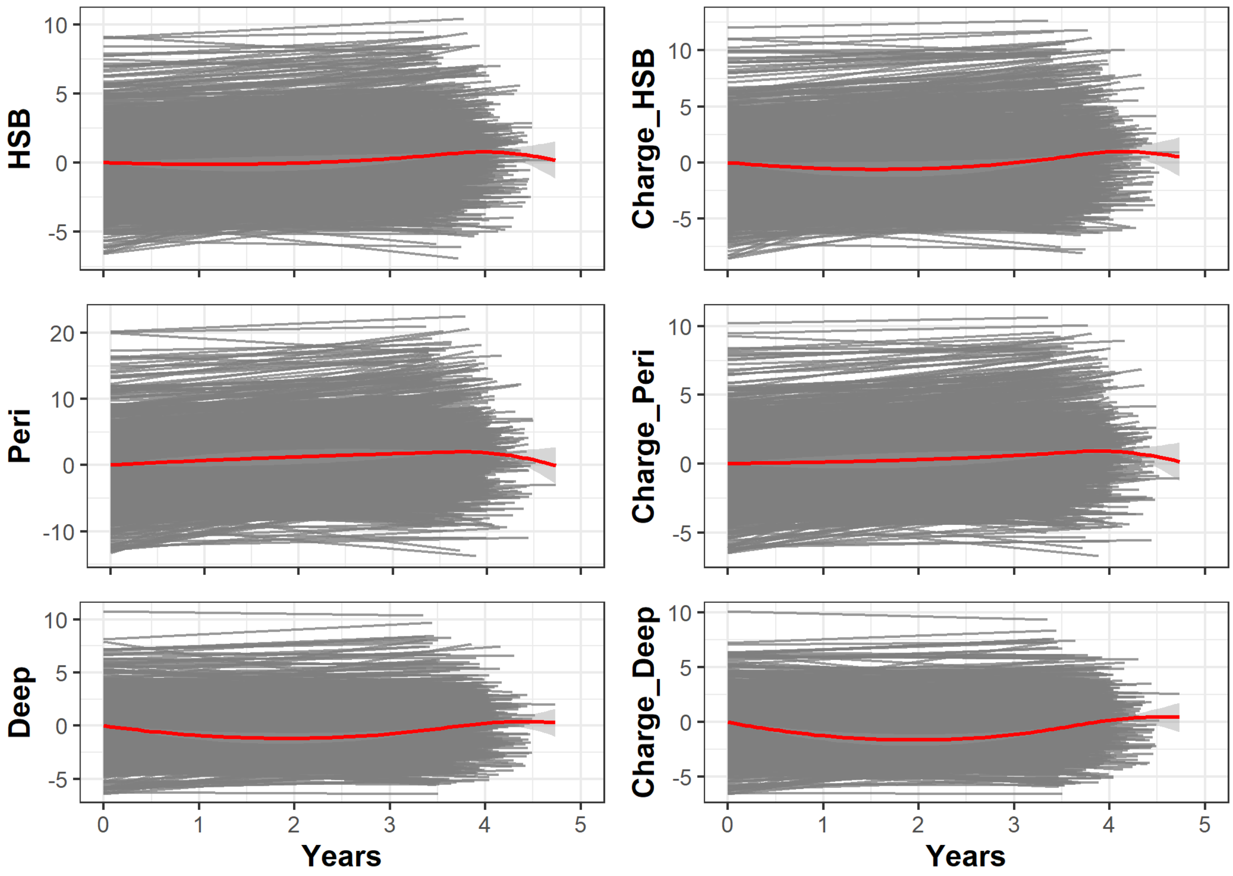


Figure 4: Individual trajectories from the normalized vascular brain-MRI predictors in the 3C study. From left to right, we display the trajectories of hypersignals volume in the white matter, proportion of hypersignals in the white matter, hypersignals volume in the periventricular white matter, proportion of hypersignals volume in the periventricular white matter, hypersignals volume in the deep white matter and proportion of hypersignals volume in the deep white matter.

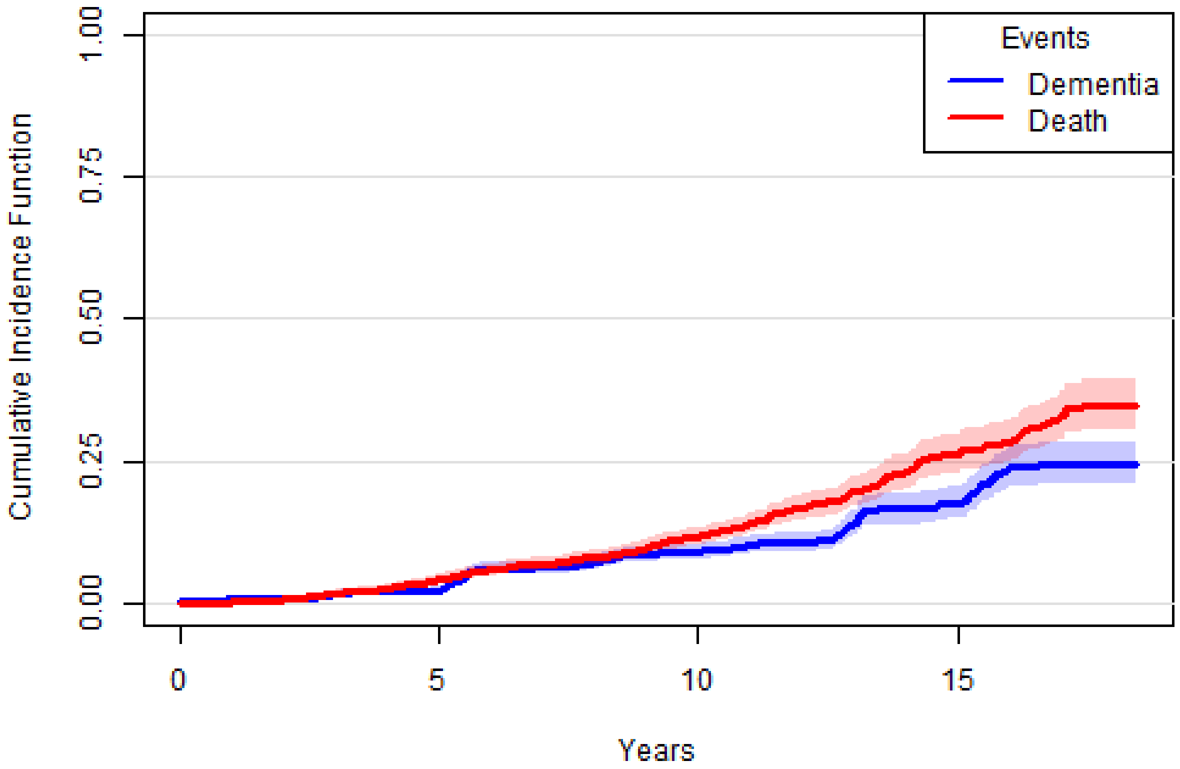


Figure 5: Cumulative incidence function for dementia (in blue) and death (in red) event over 17 years of follow-up.

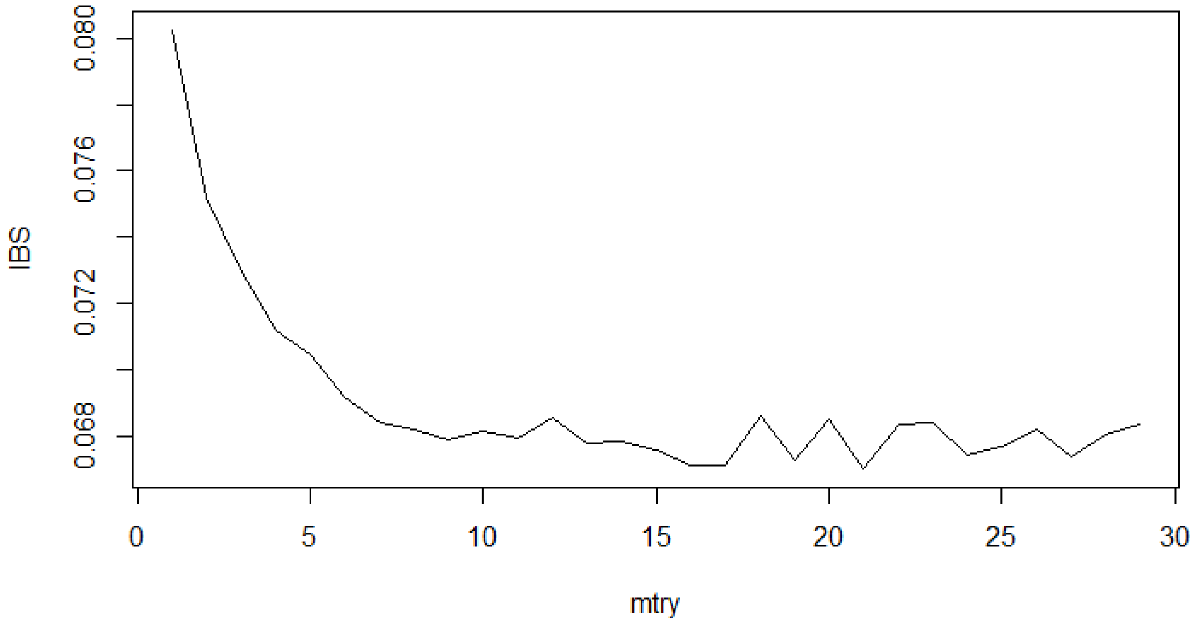


Figure 6: Integrated Brier Score (IBS) according to the range of $mtry$ parameter values from 1 to 29. Minimal IBS value was found for $mtry = 21$.

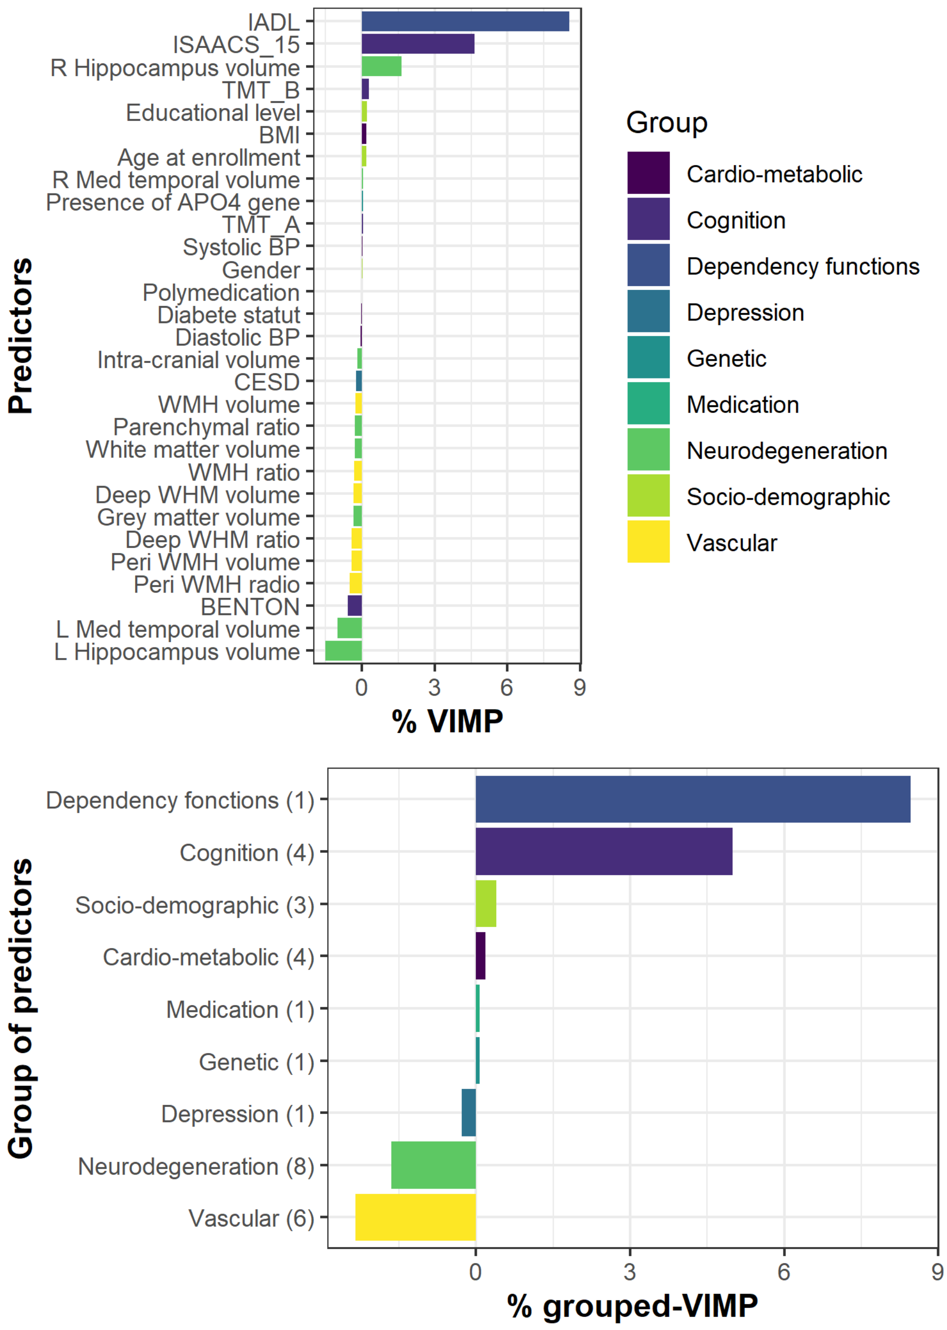


Figure 7: (A) Importance variable (VIMP) and (B) grouped importance variable (gVIMP) averaged over 10 permutation procedures for each dementia predictor or group of dementia predictors with OOB error computed between 5 and 10 years.

## Tables

Table 1: Association parameters between the markers and the time to event for the small dimension scenarios. As a reminder, $b_{02}$ indicates the baseline random-effect from the marker 2.

| **Scenario** | **Predictor** | **$\beta$ parameter** |
|---|---|---|
| Small1 | $b_{11}$ | 3 |
| | $b_{02}$ | -2 |
| | $b_{11} * b_{02}$ | -3.5 |
| Small2 | $I(c_1 = 1)$ | -2.5 |
| | $I(c_1 = 2)$ | -1 |
| | $I(c_1 = 3)$ | 1.5 |
| | $I(c_1 = 4)$ | 3 |

Table 2: Association parameters between the markers and the time to event for the large dimension scenarios. As a reminder, $b_{02}$ indicates the baseline random-effect from the marker 2.

| **Scenario** | **Predictor** | **$\beta$ parameter** |
|---|---|---|
| Large1 | $b_{01}$ | 3 |
| | $b_{12}$ | 1 |
| | $b_{13}$ | -2 |
| | $b_{15}$ | -2 |
| | $b_{01} * b_{12}$ | 2 |
| | $b_{13} * b_{15}$ | -2 |
| Large2 | $I(c_1 = 1)$ | -2 |
| | $I(c_1 = 2)$ | 2 |
| | $I(c_3 = 1)$ | -1 |
| | $I(c_3 = 3)$ | 3 |

Table 3: List of variables for the cognition group used in 3C application.

| **Abbreviation** | **Description** | **Type**$^{\star}$ |
|---|---|---|
| BENTON | Visual retention test of Benton | CTD |
| ISA_15 | Isaac Set Test | CTD |
| TMT_A | Trail Making Test A | CTD |
| TMT_B | Trail Making Test B | CTD |

$^{\star}$ CTD: Continuous Time-Dependent

Table 4: List of variables for the cardio-metabolic group used in 3C application.

| Abbreviation | Description | Type* |
|---|---|---|
| DIABBIS | Diebete status | Binary covariate |
| SBP | Systolic Blood Pressure | CTD |
| DBP | Diastolic Blood Pressure | CTD |
| BMI | Body-Mass Index | CTD |

* CTD: Continuous Time-Dependent

Table 5: List of variables for the socio-demographic group used in 3C application.

| Abbreviation | Description | Type |
|---|---|---|
| GENDER | Gender | Binary covariate |
| DIPNIV | Educational level | 5-factor covariate |
| AGE0 | Age at enrollment | Continuous covariate |

Table 6: List of variables for the neuro-degenerative group used in 3C application.

| Abbreviation | Description | Type* |
|---|---|---|
| SB | White matter volume | CTD |
| SG | Gray matter volume | CTD |
| VTI | Intracranial volume | CTD |
| PAR_FRAC | Parenchymal fraction | CTD |
| HIPP_L | Left hippocampal volume | CTD |
| HIPP_R | Right hippocampal volume | CTD |
| MED_TEMP_L | Left mediotemporal lobe volume | CTD |
| MED_TEMP_R | Right mediotemporal lobe volume | CTD |

* CTD: Continuous Time-Dependent

Table 7: List of variables for the vascular charge group used in 3C application.

| Abbreviation | Description | Type* |
|---|---|---|
| HSB | Hypersignals volume in the white matter | CTD |
| Charge_HSB | Proportion of hypersignals in the white matter | CTD |
| Peri | Hypersignals volume in the periventricular white matter | CTD |
| Charge_Peri | Proportion of hypersignals volume in the periventricular white matter | CTD |
| Deep | Hypersignals volume in the deep white matter | CTD |
| Charge_Deep | Proportion of hypersignals volume in the deep white matter | CTD |

* CTD: Continuous Time-Dependent

Table 8: List of other variables used in 3C application.

| **Abbreviation** | **Group** | **Description** | **Type**⋆ |
|---|---|---|---|
| CESDT | Depression | Depressive symtoms | CTD |
| TOT_MED | Medication | Number of drug consumed by day | CTD |
| IADL | Functional dependency | Instrumental Activities of Daily Living | CTD |
| APOE4 | Genetic | Presence of apolipoprotein e4 allel | Continuous covariate |

⋆ CTD: Continuous Time-Dependent
